# Supplementary material for: Star Clusters and Dark Matter as Probes of the Spacetime Geometry of Massive Black Holes
Source: arXiv:1308.5378 source file (2013-08-25)
Supplement: Supplementary file 1 [file AppendixTemplate.tex]

% Appendix Template

\chapter{Appendix Title Here} % Main appendix title

\label{AppendixX} % Change X to a consecutive letter; for referencing this appendix elsewhere, use \ref{AppendixX}

\lhead{Appendix X. \emph{Appendix Title Here}} % Change X to a consecutive letter; this is for the header on each page - perhaps a shortened title

Write your Appendix content here.
